# Supplementary material for: BareBones: Benchmarking Zero-Shot Geometric Comprehension in VLMs
Source: arXiv:2604.10528 source file (2026-10-05)
Supplement: Supplementary file 1 [file supp.tex]

\documentclass[10pt,twocolumn,letterpaper]{article}
\usepackage[pagenumbers]{cvpr}
\input{preamble}
\usepackage{multirow}

\definecolor{cvprblue}{rgb}{0.21,0.49,0.74}
\usepackage[pagebackref,breaklinks,colorlinks,allcolors=cvprblue]{hyperref}
\def\paperID{5}
\def\confName{CVPR}
\def\confYear{2026}

\begin{document}
% Set counters to continue from end of main paper
\setcounter{figure}{7}   % 7 figures in main → suppl starts at Fig. 8
\setcounter{table}{3}    % 3 tables in main → suppl starts at Tab. 4

\input{sec/X_suppl}
\end{document}
